# Supplementary material for: Slow noise processes in superconducting resonators
Source: arXiv:1210.2351 source file (2013-04-09)
Supplement: Supplementary file 1 [file supplemental.pdf]

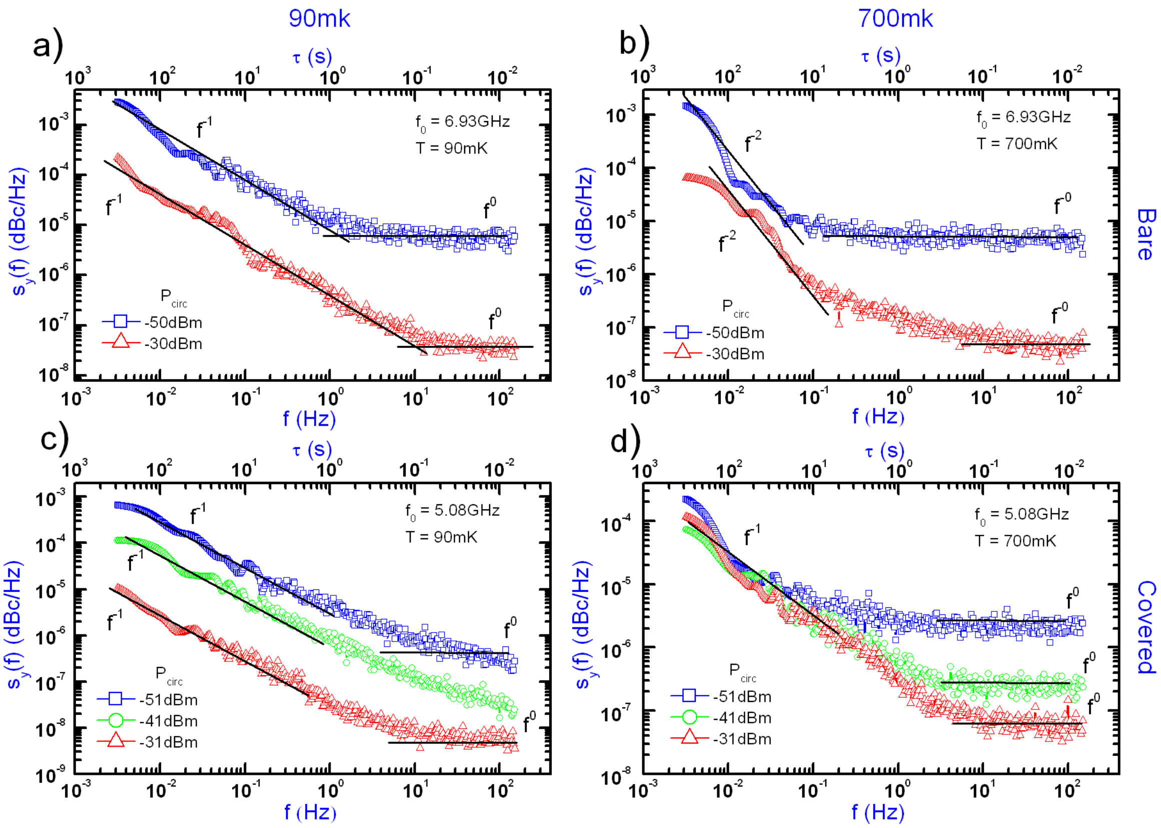


Figure 1. Spectrum of *frequency* fluctuations, expressed in dBc/Hz by the Barkhausen relation. Successive shapes correspond to different microwave drive powers, triangles = -85 dBm, circles = -95 dBm and squares = -105 dBm. Plots are of a bare resonator, B1, at 90 mk in a) and 70 0mK in b) and of an aluminum oxide covered resonator, A1, at 90 mK c) and 700 mK d). The dielectric reference oscillator is omitted for clarity

## SUPPLEMENTARY MATERIAL

To complement the Allan deviation (ADEV) plots in the article, we include PSD traces shown in figure 1. These are generated from the same data set and will be of use for readers who are more used to this way of analyzing and presenting data. The PSD and the ADEV are in many ways equivalent ways of analyzing data, and both methods lead to the same conclusions in noise type and level when fitting to the slope of the curve. However, the PSD is inherently more 'arbitrary' than the ADEV since there are many different ways of estimating the former, and no standardized methods have been agreed on (compared to the standardized ADEV method[2]). The greater averaging of the ADEV also makes more efficient use of data at low frequencies.

We used the Matlab [1] implementation of the Welch method[3] to estimate the PSD, using a Hanning window with a length of 20%, 400 lines, and a 50% overlap. All datasets have been analyzed using the same parameters. Note that the Pound method[4] produces the spectrum of frequency noise, compared to homo-dyne techniques which mostly produce the spectrum of phase noise. This is however only true above the Leeson frequency ($f_L = \nu_0/2Q$), hence the spectrum from this point rolls rapidly to a steep slope. Phase noise spectra requires the correct conversion to frequency spectra, which involves multiplication by the Fourier frequency squared, crucially this changes the slope of noise processes when converting between spectra types[5], ie. flicker frequency noise is described by $S_y \propto 1/f$ in $Hz^2/Hz$ but $S_\phi \propto 1/f^3$ in dBc/Hz. Below the Leeson frequency a Homodyne measurement will also produce the spectrum of frequency noise. In this region the Barkhausen condition can be used to express the spectrum of frequency fluctuations in different units, for example to convert from $Hz^2/Hz$ to dBc/Hz, but converting units in this way does not mean the spectrum of phase fluctuations was measured.

[1] Mathworks Inc. *See the documentation for the* `pwelch` *command.*
[2] W. Riley, NIST, Tech. Rep. 1065, 2008.
[3] P. Stoica, R. Moses, *Spectral Analysis of Signals*, Pearson Education Ltd (2005).
[4] Lindström, T., Burnett, J., Oxborrow, M., and Tzalenchuk, A. Y. Rev. Sci. Instrum. 82, 104706 (2011)
[5] E. Rubiola, Phase Noise and Frequency Stability in Oscillators (Cambridge University Press, Cambridge, England, 2009)
